# Supplementary material for: Ultrafast Switching from the Charge Density Wave Phase to a Metastable Metallic State in 1T-TiSe$_2$
Source: arXiv:2306.00311 source file (2023-06-01)
Supplement: Supplementary file 1 [file SM.pdf]

# Ultrafast switching from the charge density wave phase to a metastable metallic state in 1T-TiSe₂: supplemental material

Shaofeng Duan,[1] Wei Xia,[2] Chaozhi Huang,[1] Shichong Wang,[1] Lingxiao Gu,[1] Haoran Liu,[1] Dao Xiang,[3,4] Dong Qian,[1,4,5] Yanfeng Guo,[2] and Wentao Zhang[1,5,*]

[1]*Key Laboratory of Artificial Structures and Quantum Control (Ministry of Education), School of Physics and Astronomy, Shanghai Jiao Tong University, Shanghai 200240, China*
[2]*School of Physical Science and Technology, ShanghaiTech University, Shanghai, China*
[3]*Key Laboratory for Laser Plasmas (Ministry of Education), School of Physics and Astronomy, Shanghai Jiao Tong University, Shanghai 200240, China*
[4]*Tsung-Dao Lee Institute, Shanghai Jiao Tong University, Shanghai 200240, China*
[5]*Collaborative Innovation Center of Advanced Microstructures, Nanjing University, Nanjing 210093, China*

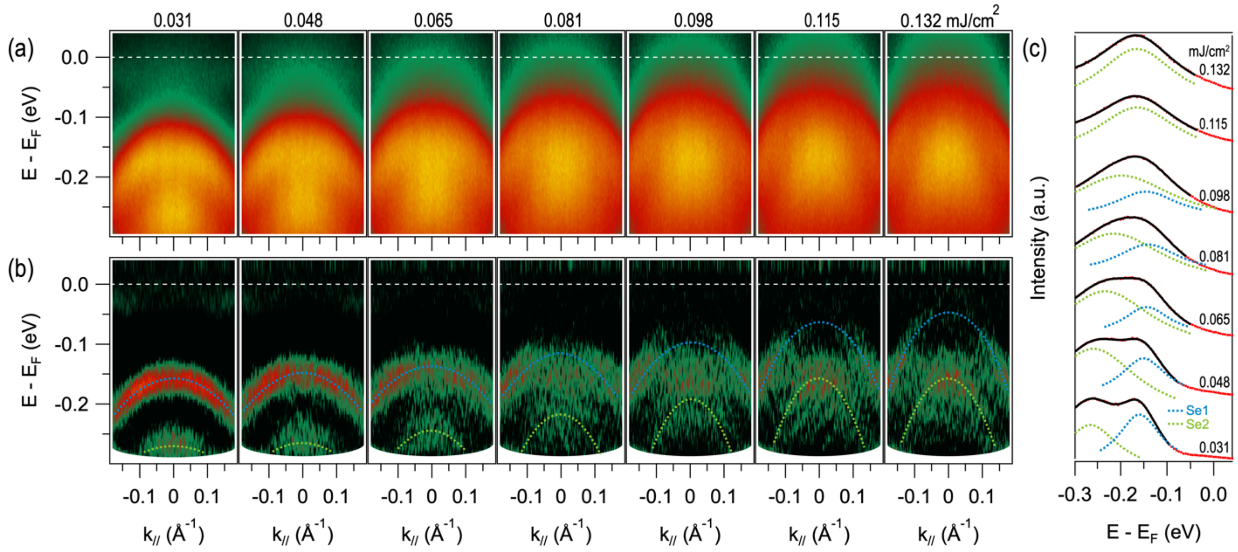


Supplemental FIG. 1. Fluence-dependent electronic structures in the CDW phase. (a) TRARPES spectra at the delay time of 0.3 ps with pump fluences of 0.031, 0.048, 0.065, 0.081, 0.098, 0.115, and 0.132 mJ/cm$^2$ and (b) the corresponding second-derivative images. (c) Energy distribution curves at Γ point from (a). The dotted lines are the Lorentzian fitting curves to capture the peak positions of the Se1 and Se2 bands. The black solid lines are the sum of the fitting results of the Se1 and Se2 bands.

*wentaozhang@sjtu.edu.cn

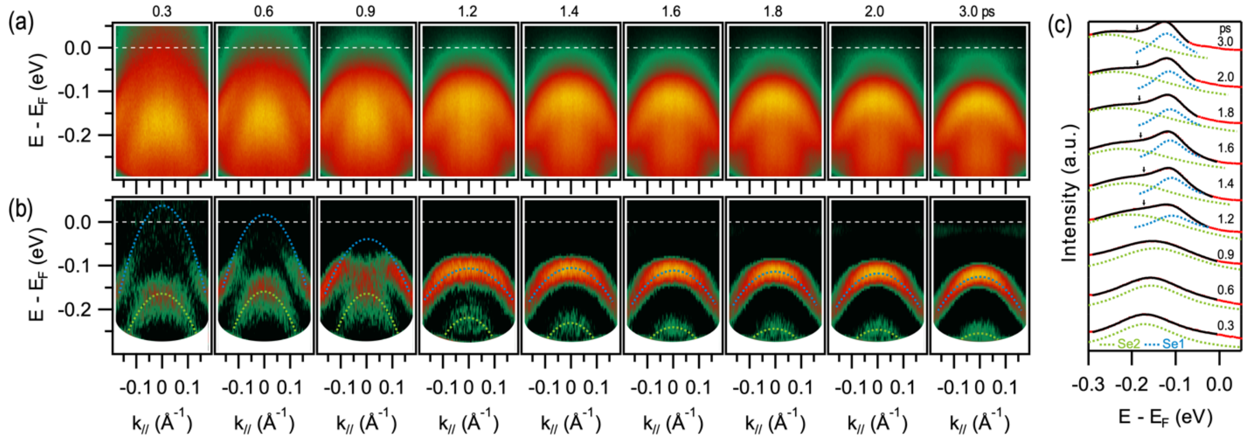


Supplemental FIG. 2. Time-dependent electronic structures in the CDW phase at pump fluence of 0.356 mJ/cm$^2$ with better energy resolution. (a) TRARPES spectra at the delay time of 0.3, 0.6, 0.9, 1.2, 1.4, 1.6, 1.8, 2.0, and 3.0 ps with pump fluences of 0.356 mJ/cm$^2$ and (b) the corresponding second-derivative images. (c) Energy distribution curves at Γ point from (a). The dotted lines are the Lorentzian fitting curves to capture the peak positions of the Se1 and Se2 bands. The black solid lines are the sum of the fitting results of the Se1 and Se2 bands. The black arrows indicate the dip feature.

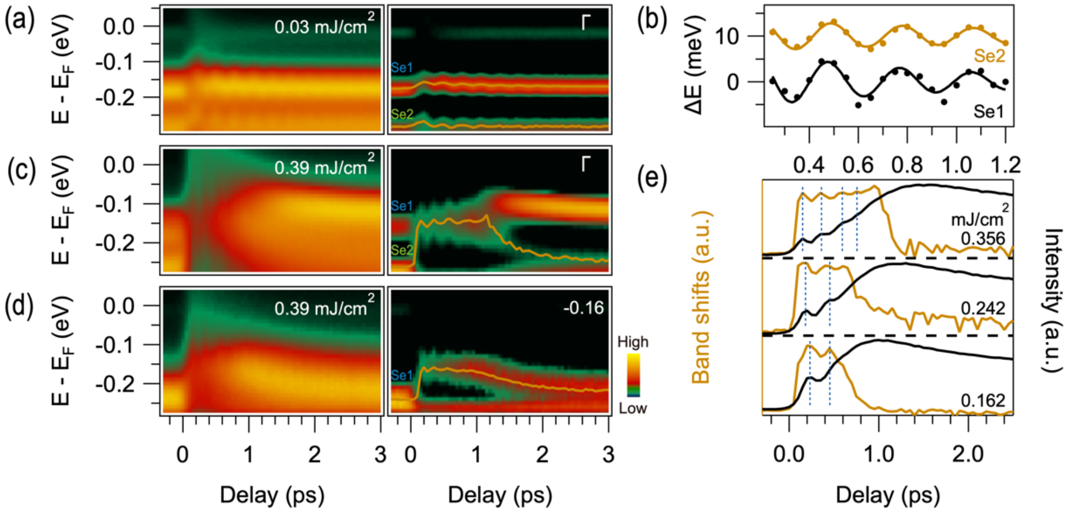


Supplemental FIG. 3. Ultrafast electronic dynamics in the CDW phase at an equilibrium temperature of 4 K. (a) Time-dependent photoemission spectra (left) and its corresponding second-derivative images (right) at Γ point for the pump fluence at 0.03 mJ/cm$^2$. The orange solid lines indicate the peak positions of the Se1 and Se2 bands obtained by Lorentzian fitting. (b) Ultrafast dynamics of Se1 and Se2 bands after subtracting smooth backgrounds (dotted lines, 10 meV offset for better illustration). The solid lines represent the fits of the data. (c) and (d) Time-dependent photoemission spectra (left) and the corresponding second-derivative images (right) at Γ point and momentum of -0.16 Å$^{-1}$ for the pump fluence at 0.39 mJ/cm$^2$. The orange solid lines indicate the peak positions of the Se2 and Se1 valence bands, respectively. (e) Time-dependent binding energies of the Se2 band and spectral intensity integrated from the band top of the Se1 band to the Fermi level at the selected pump fluence.

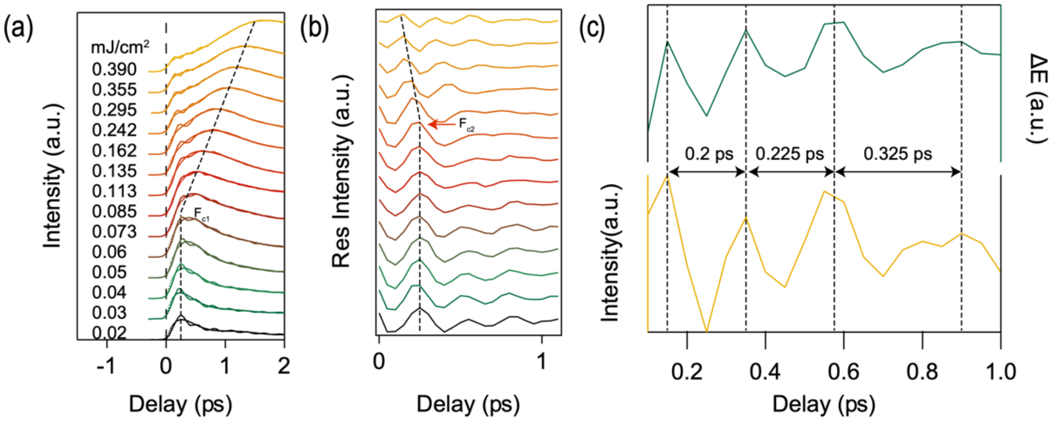


Supplemental FIG. 4. (a) Pump-fluence-dependent spectral intensity as a function of the delay time integrated from −0.1 eV (Se1 $4p_{x,y}$ band top) to the Fermi energy and (b) residual intensities after removing smooth backgrounds from the curves shown in (a). (c) Residual spectral intensity (bottom, yellow line) and energy shifts of the Se2 band (top, green line) at pump fluence of 0.39 mJ/cm$^2$ with delay times from 0.1 to 1 ps. The black arrows indicate the distance between the adjacent peaks.

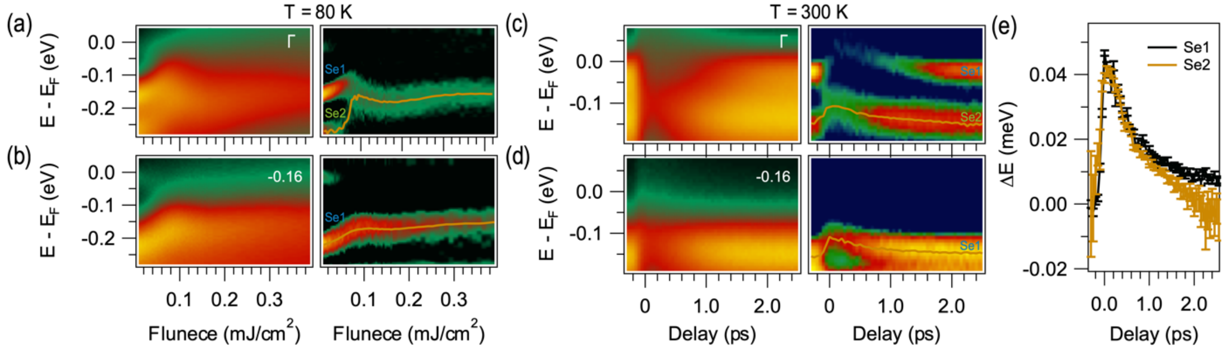


Supplemental FIG. 5. Ultrafast electronic dynamics of valence bands at temperatures of 80 and 300 K. (a) and (b) Fluence-dependent photoemission spectra at Γ and momentum of -0.16 Å$^{-1}$ measured at 80 K, and their corresponding second-derivative images along the energy axis (right) for the pump fluence at 0.39 mJ/cm$^2$. (c) and (d) Time-dependent photoemission spectra at Γ point and momentum of -0.16 Å$^{-1}$ measured at 300 K, and their corresponding second-derivative images along the energy axis (right) for the pump fluence at 0.39 mJ/cm$^2$. The orange solid lines indicate the peak positions of the Se1 and Se2 valence bands. (e) Photoinduced band shifts of the Se1 and Se2 bands as a function of delay time.

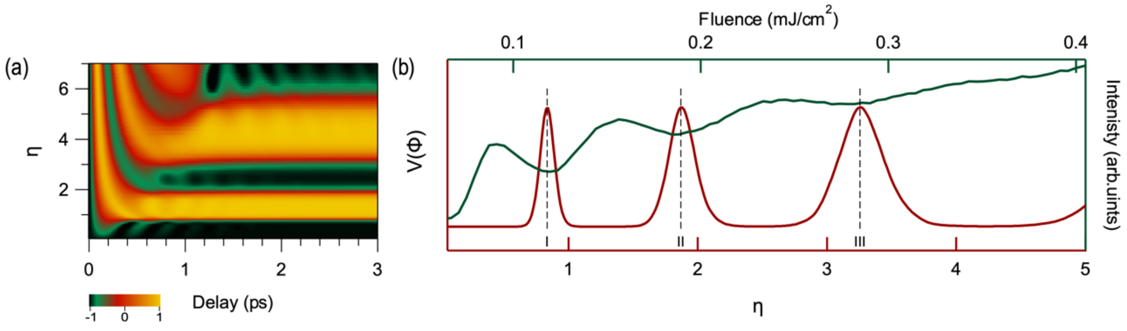


Supplemental FIG. 6. (a) Simulated order parameter at the sample surface ($z = 0$) as functions of delay time and pump fluence $\eta$. (b) Calculated fluence-dependent Ginzburg-Landau potential (crimson line) at delay time 3 ps and spectral intensity (green line) at delay

time 12 ps integrated from -0.1 eV (Se1 band top) to the Fermi Level.

**Supplemental Discussion #1**

From previous photon energy-dependent electronic structures measurements [S1], there are six low-energy bands located at the Brillouin-zone center Γ point, including two A-derived Se $4p_{x,y}$ bands, two Γ-derived Se $4p_{x,y}$ bands, one Γ-derived Se $4p_z$ band, and one L-derived Ti $3d_{z^2}$ conduction band. After photoexcitation, the folded bands from A and L points disappeared due to the destruction of the period lattice distortions, and they were partially restored at long delay times of about 12 ps in our previous study [S2]. However, the spectral intensity of these folded bands is too weak to be tracked in the photoinduced metallic metastable state within 1 ps. In addition, we have tried to change the polarization of the probe beam, but there was no observable Se $4p_z$ band in our ARPES experiments, which was possibly due to the photoemission matrix element effect.

**Supplemental Discussion #2**

In Supplemental FIG. 1, we showed detailed pump-fluence-dependent electronic structures at a delay time of 0.3 ps. It is clear that the Se2 bands gradually shift up by about 85 meV toward the Fermi energy with increasing the pump fluences up to near 0.098 mJ/cm$^2$. Above the melting threshold of the CDW order, the band top of the Se1 band could not be well defined and the Se2 band is nearly located at the unperturbed binding energy of the Se1 band within the first ps, as shown in Figs. 1(b) and 1(d) in the main text. Therefore, the EDC peaks within the 1 ps in panels (c) and (e) are attributed to the Se2 valence band. The vanished band top of the Se1 band after melting the CDW order was possibly due to the strong excitonic fluctuation and matrix element effects in photoemission.

**Supplemental Discussion #3**

To better illustrate the ultrafast recovery dynamics of the Se2 band, we took additional time-dependent electronic structure measurements with better energy resolution by compromising the time resolution of the TRARPES system. In Supplemental FIG. 2, we showed the time-dependent electronic structures at selected delay times with a pump fluence of 0.356 mJ/cm$^2$. After photoexcitation within 1 ps, the Se1 band top could not be well defined and the Se2 band showed obvious energy shifts toward the Fermi energy, which were consistent with our observations in the main text. After about 1 ps, the intensity of the Se1 band top recovered and the Se2 band showed obvious downward shifts, gradually recovering to its equilibrium state at longer delay times. The energy distribution curves at Γ point showed anomalous peak-dip-hump line shape and a dip feature appeared in the EDCs after the delay time of 1.2 ps (Supplemental FIG. 2(c)). The spectral intensity could be fitted with two Lorentz functions plus a linear background after 0.9 ps

$$I(E) = \sum_{i=1,2} \frac{I_i}{(E-E_i)^2+{w_i}^2} + I_3 + I_4 \times E\ .$$

Here $E_i$ and $w_i$ represent the position and width of the peak, respectively. However, the broad EDCs of both the Se1 and Se2 bands between 1 and 1.5 ps make it difficult to precisely get the peak position shown in the revised Fig. 2(c). After about 1.5 ps, the spectral intensity of the Se2 band gradually enhanced, and the peak positions in the EDCs could be well defined.

**Supplemental Discussion #4**

In the weak-excitation regime, ultrafast optical excitations induce the coherent phonons, which periodically modulate the electronic states and can be captured by time- and angle-resolved photoemission spectroscopy (trARPES). Supplemental FIG. 3(a) showed the time-dependent photoemission spectrum at the Brillouin center Γ point with a pump fluence of 0.03 mJ/cm$^2$ in the CDW state, and coherent oscillations can be identified in both the intensity and energy shifts of the Se1 and Se2 $4p_{x,y}$ bands. The orange solid lines in Supplemental FIG. 3(a) indicate the time-dependent binding energies, which are directly coupled to the coherent phonon mode in $TiSe_2$. After subtracting smooth backgrounds, the residual band shifts show obvious coherent oscillations (Supplemental FIG. 3(b)), which can be nicely fitted to an exponentially decaying cosine function

$$f(t) = A * \exp(-t/\tau) * \cos{(2\pi\omega t + \phi)},$$

in which $\omega$ is the coherent phonon frequency, $\phi$ is the initial phase. $A$ and $\tau$ represent the oscillation amplitude and the relaxation time constant, respectively. The extracted oscillation frequency of Se1 and Se2 bands are 3.44 ± 0.02 THz and 3.41 ± 0.05 THz, which corresponds to the $A_{1g}^*$-CDW amplitude mode and is consistent with previous experiments [S3-S7].

In the strong-excitation regime, ultrafast excitation induces an instantaneous modification of free energy by photoinduced quasiparticle populations. Time-dependent Ginzburg-Landau model simulations show that the lifetime of this light-induced metastable state in $TiSe_2$ is dependent on the incident pump fluence. To better visualization of the plateau feature and the anharmonic oscillations after melting the CDW order, we performed the ultrafast electronic structure measurements with a pump fluence beyond the highest excitation density of 0.356 mJ/cm$^2$ in the main text. Upon increasing the pump fluence of 0.39 mJ/cm$^2$, the CDW order was quickly quenched

after infrared photoexcitation. The plateau features and anharmonic oscillations show up in the time-dependent binding energies of both Se1 and Se2 bands, as shown in Supplemental FIGs. 3(c) and (d). The anharmonic oscillations also appear in the time-dependent spectral intensity integrated between the band top of the Se1 valence band and the Fermi level [S2]. In Supplemental FIG. 3(e), we compare the time-dependent binding energies of the Se2 band with the spectral intensity at selected pump fluences, and the oscillations in both are in the same frequency and phase. Such anharmonic oscillations are signatures of forced vibration, and the system can be driven to its normal phase or even inverted states after several picoseconds.

**Supplemental Discussion #5**

In supplemental FIG. 4, we showed the time-dependent spectral intensity at Γ point integrated from the binding energy -0.1 eV (Se1 $4p_{x,y}$ band top) to the Fermi energy and their corresponding residual intensity after subtracting smooth backgrounds. At low pump fluence below $F_{c1}$, the time-dependent spectral intensity clearly showed coherent oscillations, which was the result of photoinduced $A_{1g}$-CDW phonons. The coherent oscillations were also shown in the binding energy of the Se1 and Se2 bands (Figs. 2(d) and (e) in the main text). At high pump fluence above $F_{c2}$, the spectral intensity oscillations occurred immediately after time zero, and the peak-to-peak distances were shorter than the period of the $A_{1g}$-CDW phonon modes, which demonstrated the Ginzburg-Landau potential was transiently changed after photoexcitation and became time-dependent, giving the motion of the order parameter in an anharmonic way. The anharmonic oscillations at high pump fluences mean that the motion of the order parameter and the corresponding atoms are still coherent but without a certain frequency. Such anharmonic oscillations can be clearly evidenced by the fact that the adjacent peak-to-peak distances of the residual intensity and time-dependent energy shifts of the Se2 band became wider at longer delay times (Supplemental FIG. 4(c)).

**Supplemental Discussion #6**

Supplemental FIGs. 5(a) and (b) show the fluence-dependent photoemission spectra at Γ point and momentum of -0.16 $\text{Å}^{-1}$ and their corresponding second-derivative images at equilibrium temperature 80 K. The fluence-dependent energy shifts of Se1 and Se2 bands monotonously increase below the critical fluence $F_c$. Above $F_c$, the binding energies of Se1 and Se2 bands are nearly fluence-independent, and it is consistent with the ultrafast electronic dynamics at temperature 4 K. Supplemental FIGs. 5(c) and (d) show the time-dependent photoemission spectra in the normal phase of temperature 300 K. To quantitatively compare with the valence band dynamics in the CDW phase, we focus on the evolution of the Se2 band at Γ point and Se1 band at the momentum of -0.16 $\text{Å}^{-1}$. Distinct from previous studies [S7], the better separation of the Se1 and Se2 bands due to the improved experimental resolution allows us to track the dynamics of the two valence bands. The binding energies of both Se1 and Se2 bands exhibit clear upshifts after photoexcitation and then quickly recovered to their equilibrium values exponentially (Supplemental FIG. 5(e)). It seems that the photoexcitation in the normal phase merely serves to reach much higher electron temperatures and the ultrafast dynamics of the valence bands are just the results of heated electronic states by ultrafast photoexcitation. The apparent difference between the ultrafast electronic dynamics in the normal phase and the CDW state demonstrates that the light-induced metastable state is not a result of the laser-induced heating effect.

**Supplemental Discussion #7**

The ultrafast dynamics of the order parameter are determined by the motion equation derived from the time-dependent double-well Ginzburg-Landau potential in the main text. The motion equation of the order parameter is

$$\frac{1}{\omega_0^2}\frac{\partial^2}{\partial t^2}\Phi + \frac{\gamma}{\omega_0}\frac{\partial}{\partial t}\Phi - \frac{1}{2}\left[1 - \eta\exp\left(-\frac{t}{\tau_e}\right)\exp\left(-\frac{z}{z_p}\right)\right]\Phi + \frac{1}{2}\Phi^3 - \frac{\xi^2}{2}\frac{\partial^2}{\partial z^2}\Phi = 0,$$

in which $\omega_0$ is the frequency of the CDW coherent phonon mode, $\gamma = 0.2$ is the phenomenological damping coefficient, and other coefficients are described in the main text. The above equation does not have an analytical expression, numerical solutions of the motion equation are described in Ref. [S2]. The ultrafast dynamics of the order parameter (Figs. 4(a)-(c) in the main text) can be obtained by solving the motion equation with the input of the above parameters in $TiSe_2$.

**Supplemental Discussion #8**

After about 1 ps, the photoinduced metallic metastable state disappeared and the system would enter into its original or inverted phase at longer delay times [S2]. Although trARPES is not able to directly distinguish the original and inverted phase from time-dependent electronic structures, it could indirectly determine the final state of the system at specific pump fluence from fluence-dependent electronic structure measurements. From our previous studies, we found that the pump laser would induce order parameter inversion sectionally inside the sample with two-dimensional (2D) interfaces established parallel to the sample surface at the interval between the inverted phase and the original phase [S2]. By finely increasing the pump fluence, the 2D interface can be positioned near the

sample surface alternately (Supplemental FIG. 6(a)). Based on the Ginzburg-Landau simulation, we found the 2D interface will be located near the sample surface ($z$=0) at pump fluences of $\eta$ = 0.8, 1.9, and 3.2, and experimentally the fluence-dependent spectral intensity and spectral linewidth show obvious dip features at fluences of 0.116, 0.185, and 0.273 mJ/cm$^2$ (denoted by I, II, and III). By comparing the fluence-dependent electronic structures with the calculated Ginzburg-Landau potential, we can indirectly determine which state (original or inverted) the systems enter into from the detail fluence-dependent electronic measurements at long delay times (Supplemental FIG. 6(b)). It should be noted that the system will not be able to fully recover to its original state ($\Phi = -1$) or inverted state ($\Phi = +1$) at specific pump fluence and there are continuously intermediate phases between $\Phi = -1$ and $\Phi = +1$ when considering the effect of the CDW coherent length. In addition, the probe photon energy of 6.05 eV in our studies will enhance the bulk sensitivity in ARPES experiments and it could probe the top 4-5 layers of the unit cell, making it hard to precisely determine which state the systems finally enter into. Nonetheless, we can roughly conclude that the sample surface enters into the original phase for the pump fluences of 0.03, 0.04, 0.06, 0.073, 0.085, and 0.242 mJ/cm$^2$, and the inverted phase for pump fluences of 0.113, 0.135, 0.162, 0.295, and 0.356 mJ/cm$^2$ by comparing the fluence-dependent electronic structures with the calculated Ginzburg-Landau potential (Supplemental FIG. 6(b)).


[S1] M. D. Watson, O. J. Clark, F. Mazzola, I. Marković, V. Sunko, T. K. Kim, K. Rossnagel, and P. D. C. King, Physical Review Letters 122, 076404 (2019).

[S2] S. Duan, Y. Cheng, W. Xia, Y. Yang, C. Xu, F. Qi, C. Huang, T. Tang, Y. Guo, W. Luo, D. Qian, D. Xiang, J. Zhang, and W. Zhang, Nature 595, 239 (2021).

[S3] E. Möhr-Vorobeva, S. L. Johnson, P. Beaud, U. Staub, R. De Souza, C. Milne, G. Ingold, J. Demsar, H. Schaefer, and A. Titov, Physical Review Letters 107, 036403 (2011).

[S4] C. S. Snow, J. F. Karpus, S. L. Cooper, T. E. Kidd, and T.-C. Chiang, Physical Review Letters 91, 136402 (2003).

[S5] J. A. Holy, K. C. Woo, M. V. Klein, and F. C. Brown, Physical Review B 16, 3628 (1977).

[S6] M. Porer, U. Leierseder, J.-M. Ménard, H. Dachraoui, L. Mouchliadis, I. E. Perakis, U. Heinzmann, J. Demsar, K. Rossnagel, and R. Huber, Nature Materials 13, 857 (2014).

[S7] H. Hedayat, C. J. Sayers, D. Bugini, C. Dallera, D. Wolverson, T. Batten, S. Karbassi, S. Friedemann, G. Cerullo, J. van Wezel, S. R. Clark, E. Carpene, and E. Da Como, Physical Review Research 1, 023029 (2019).
